# Supplementary material for: Growth and crystallographic structure of TiTe$_2$ on Au(111): From sub-monolayer structures to single- and multi-layer films
Source: arXiv:2602.16647 ancillary file (2026-02-18)

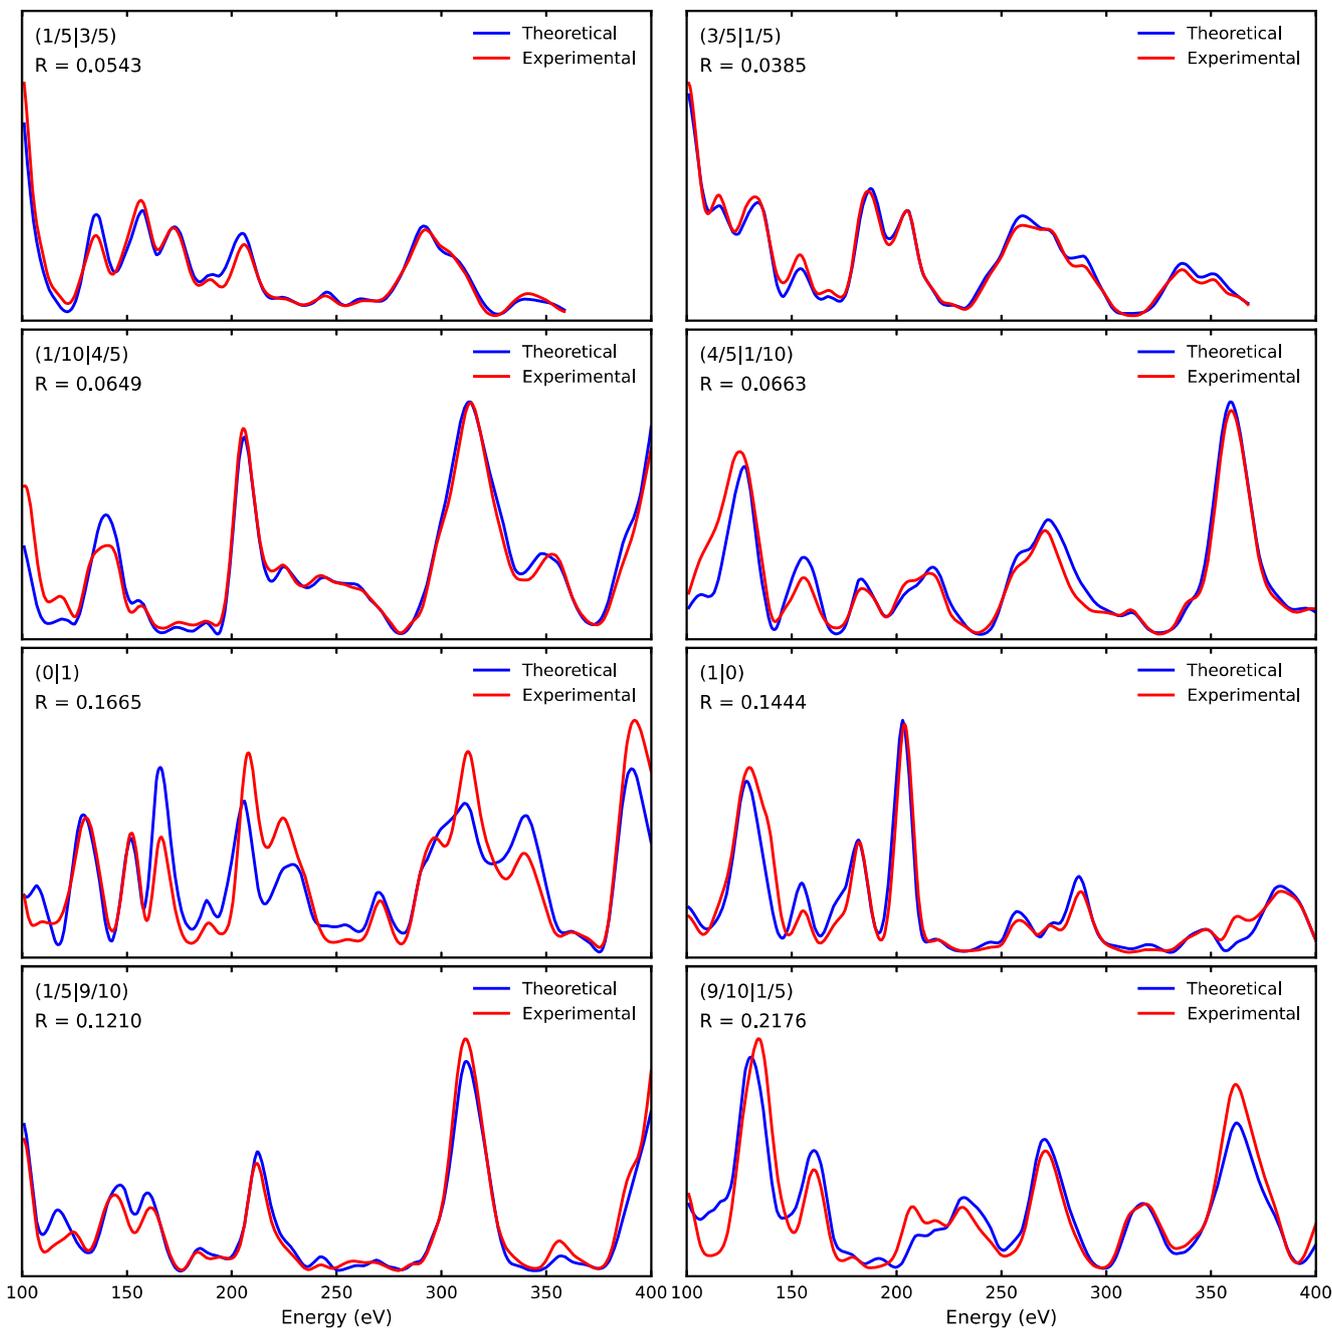

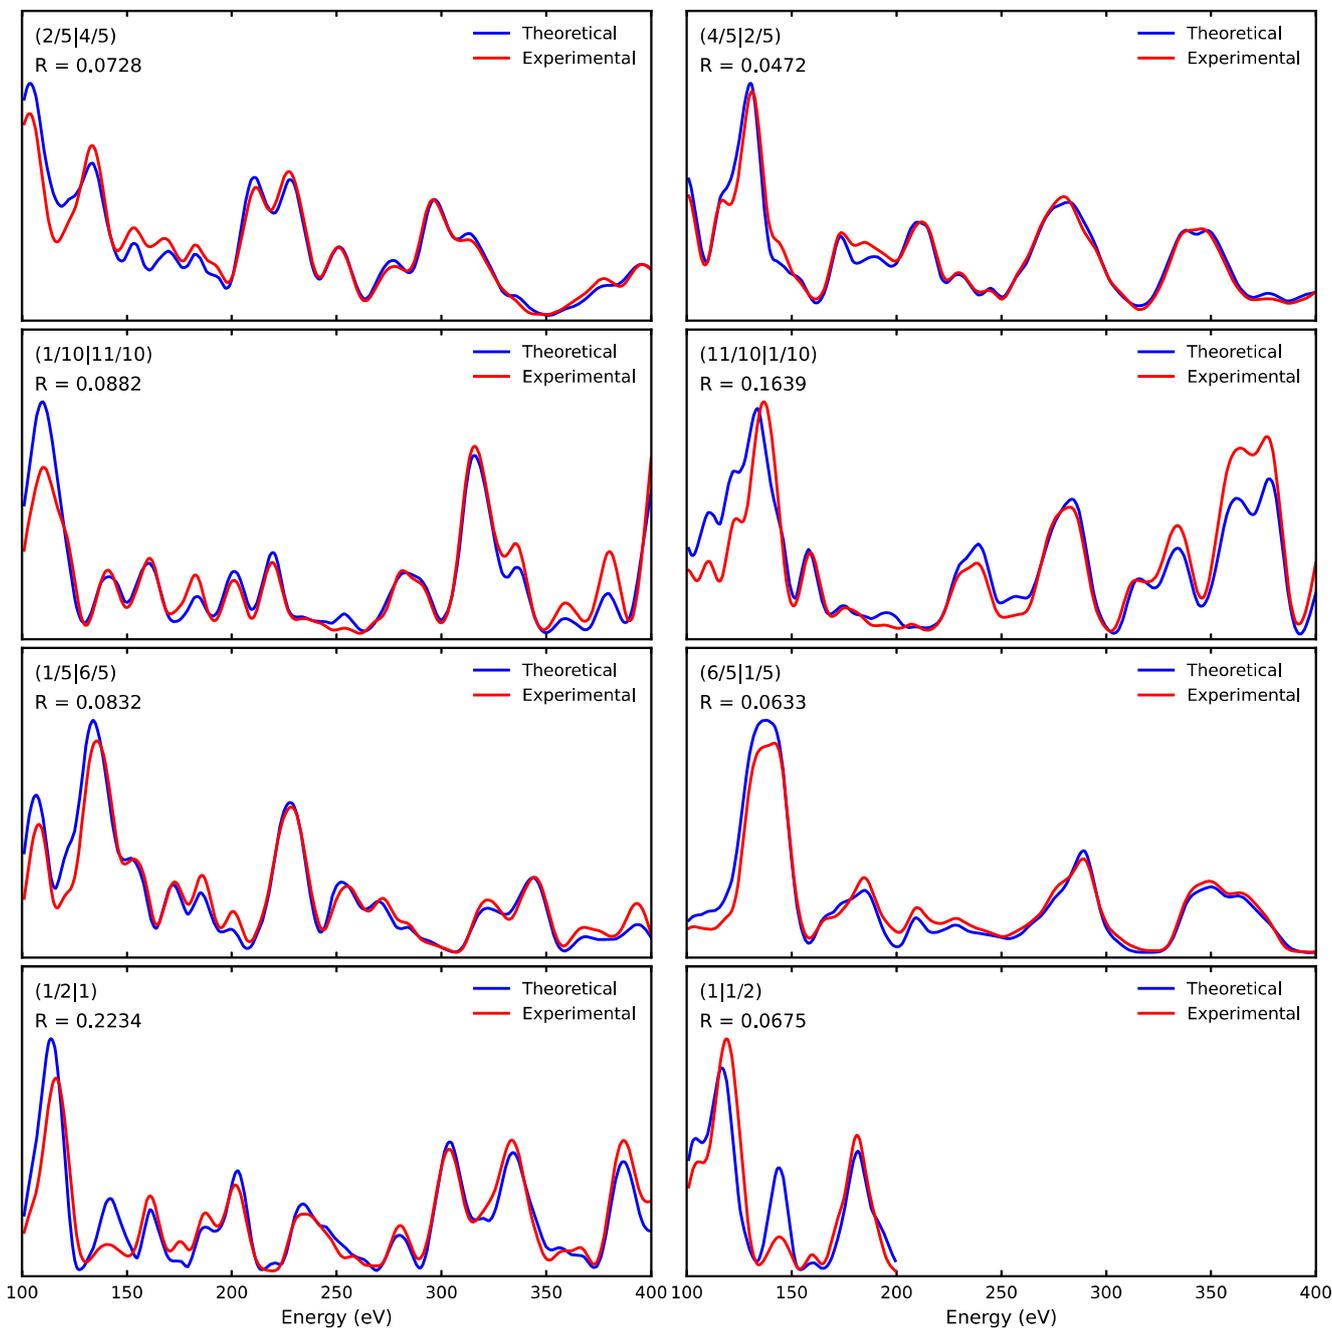

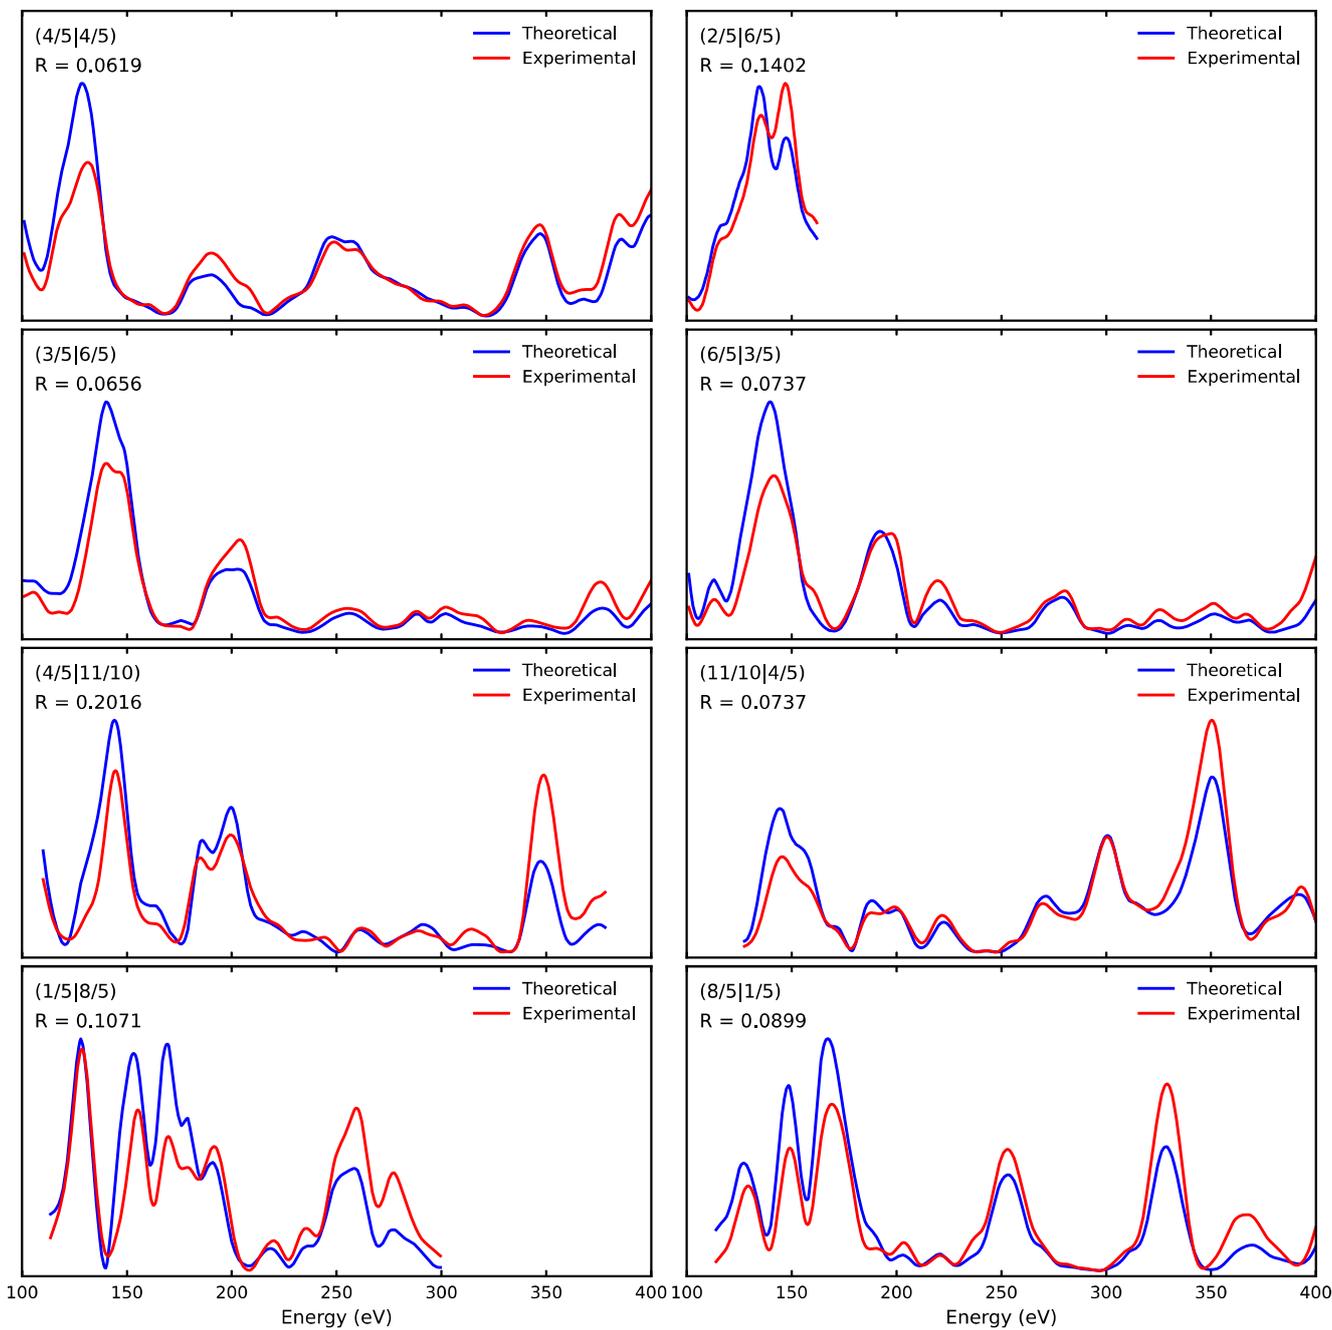

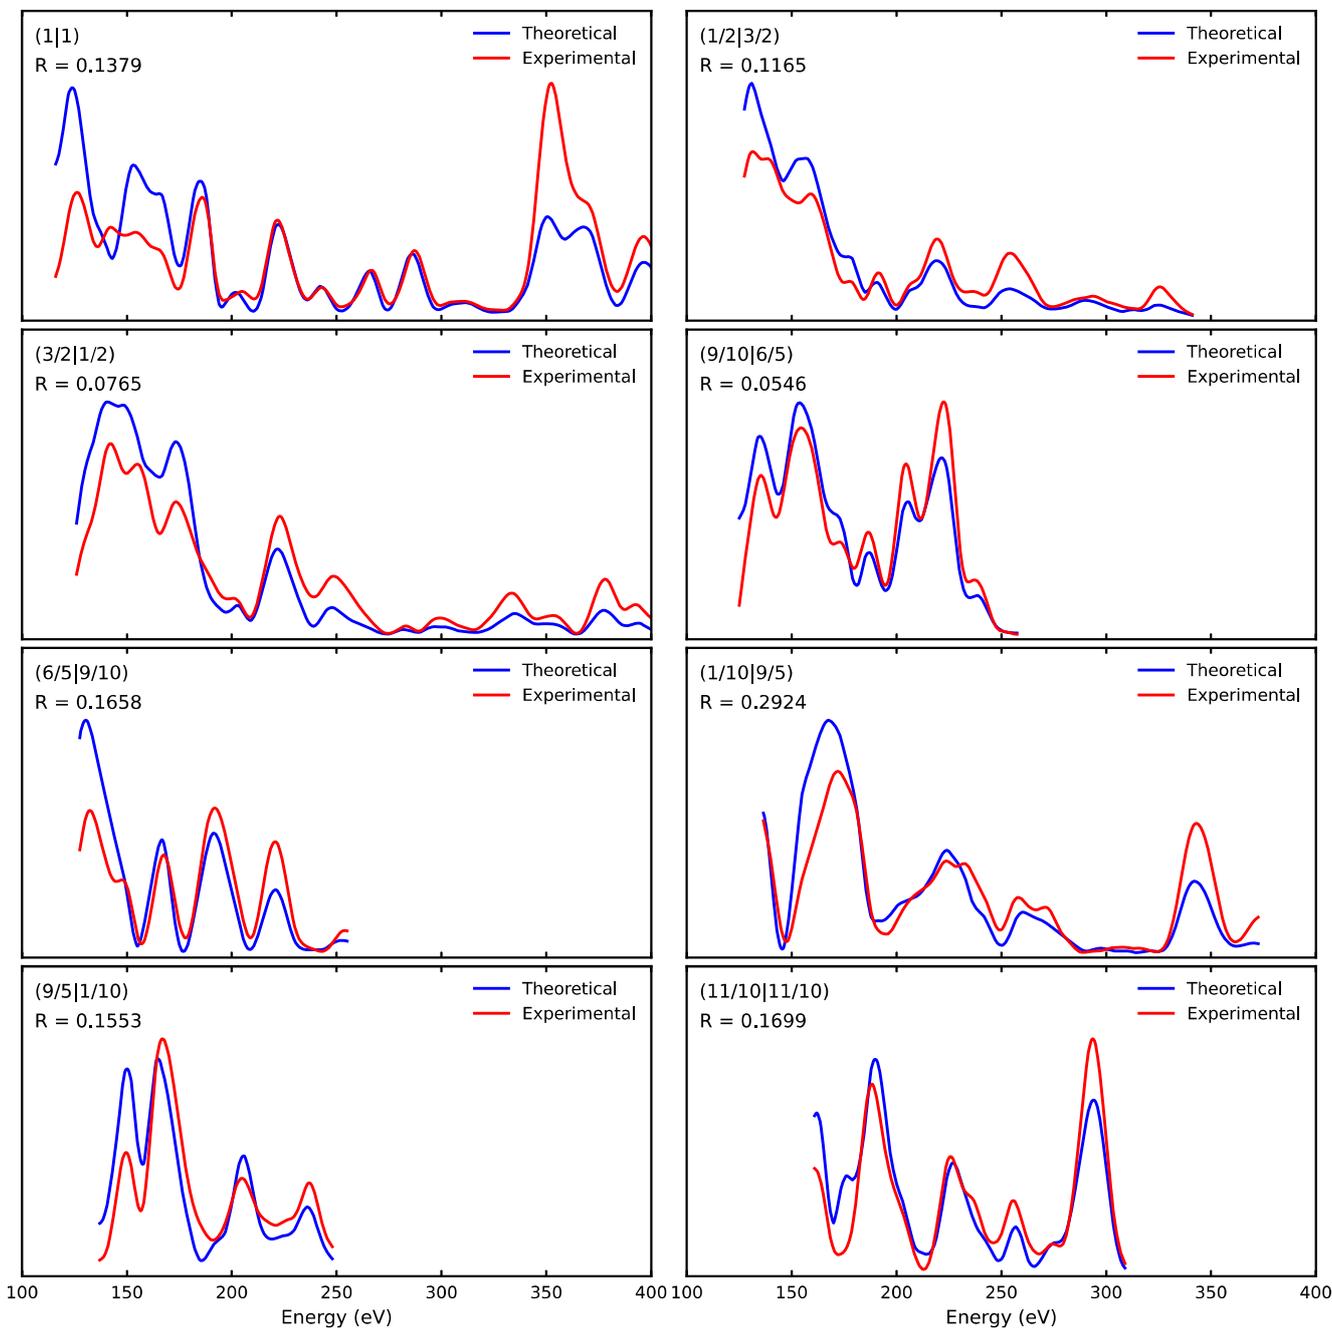

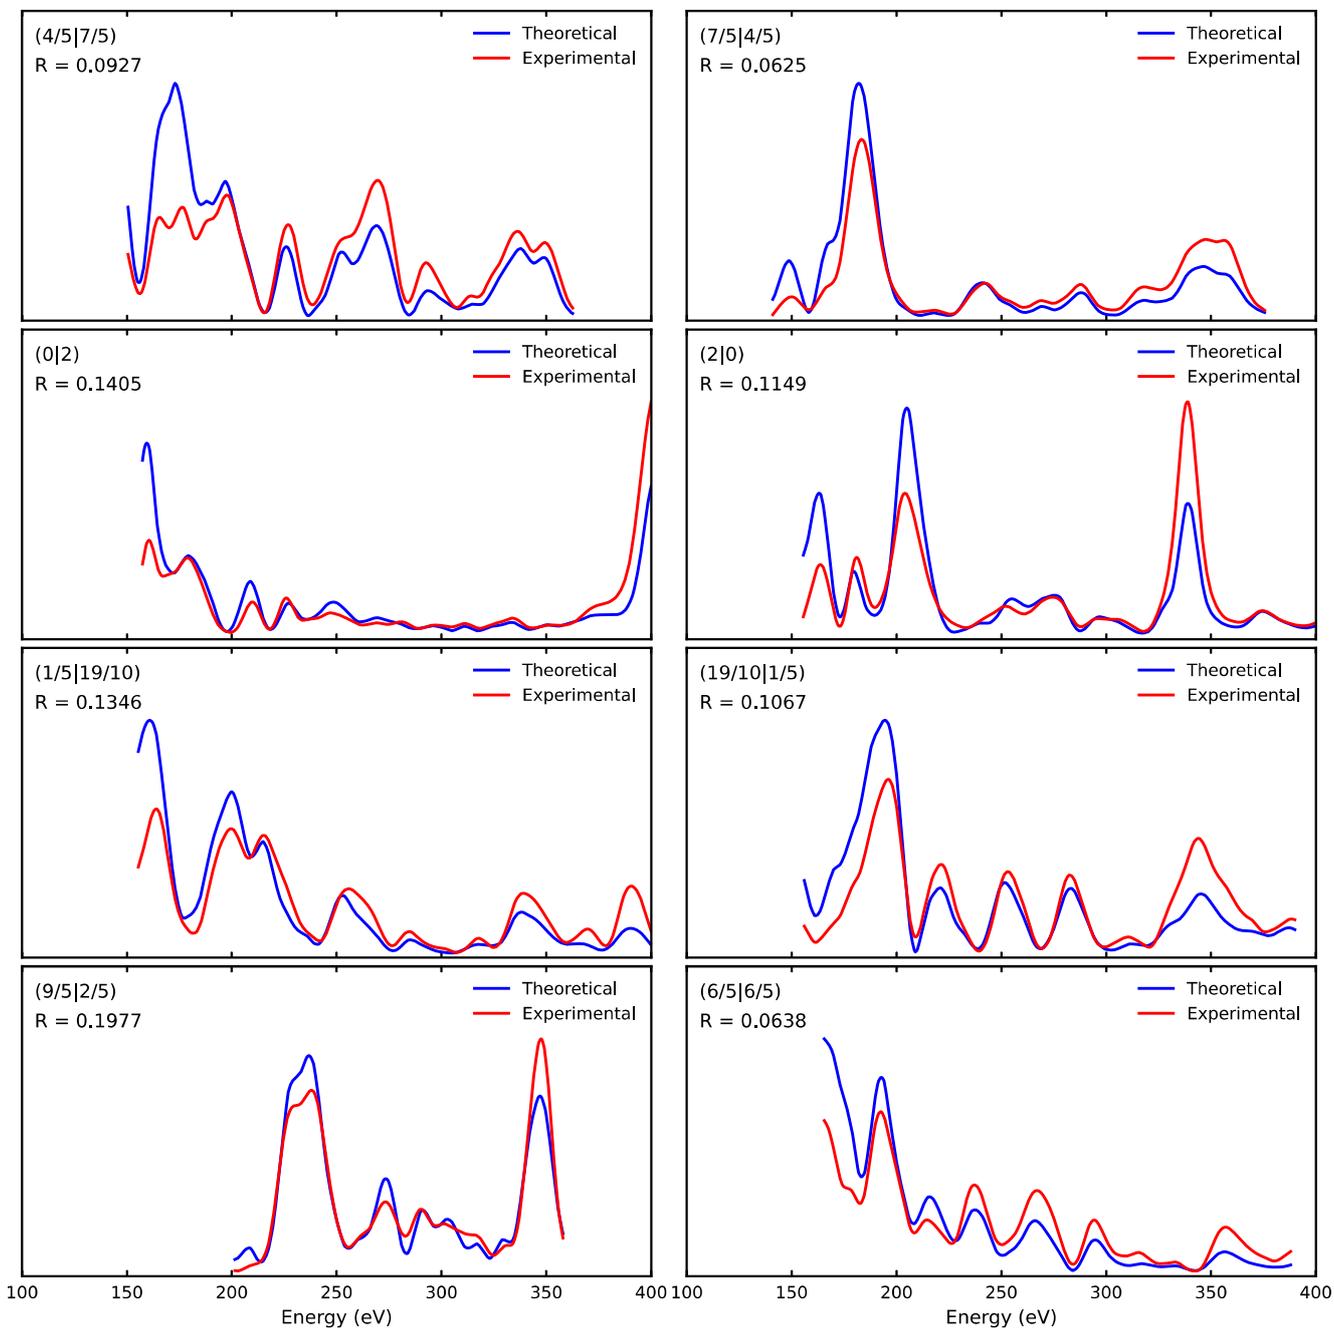

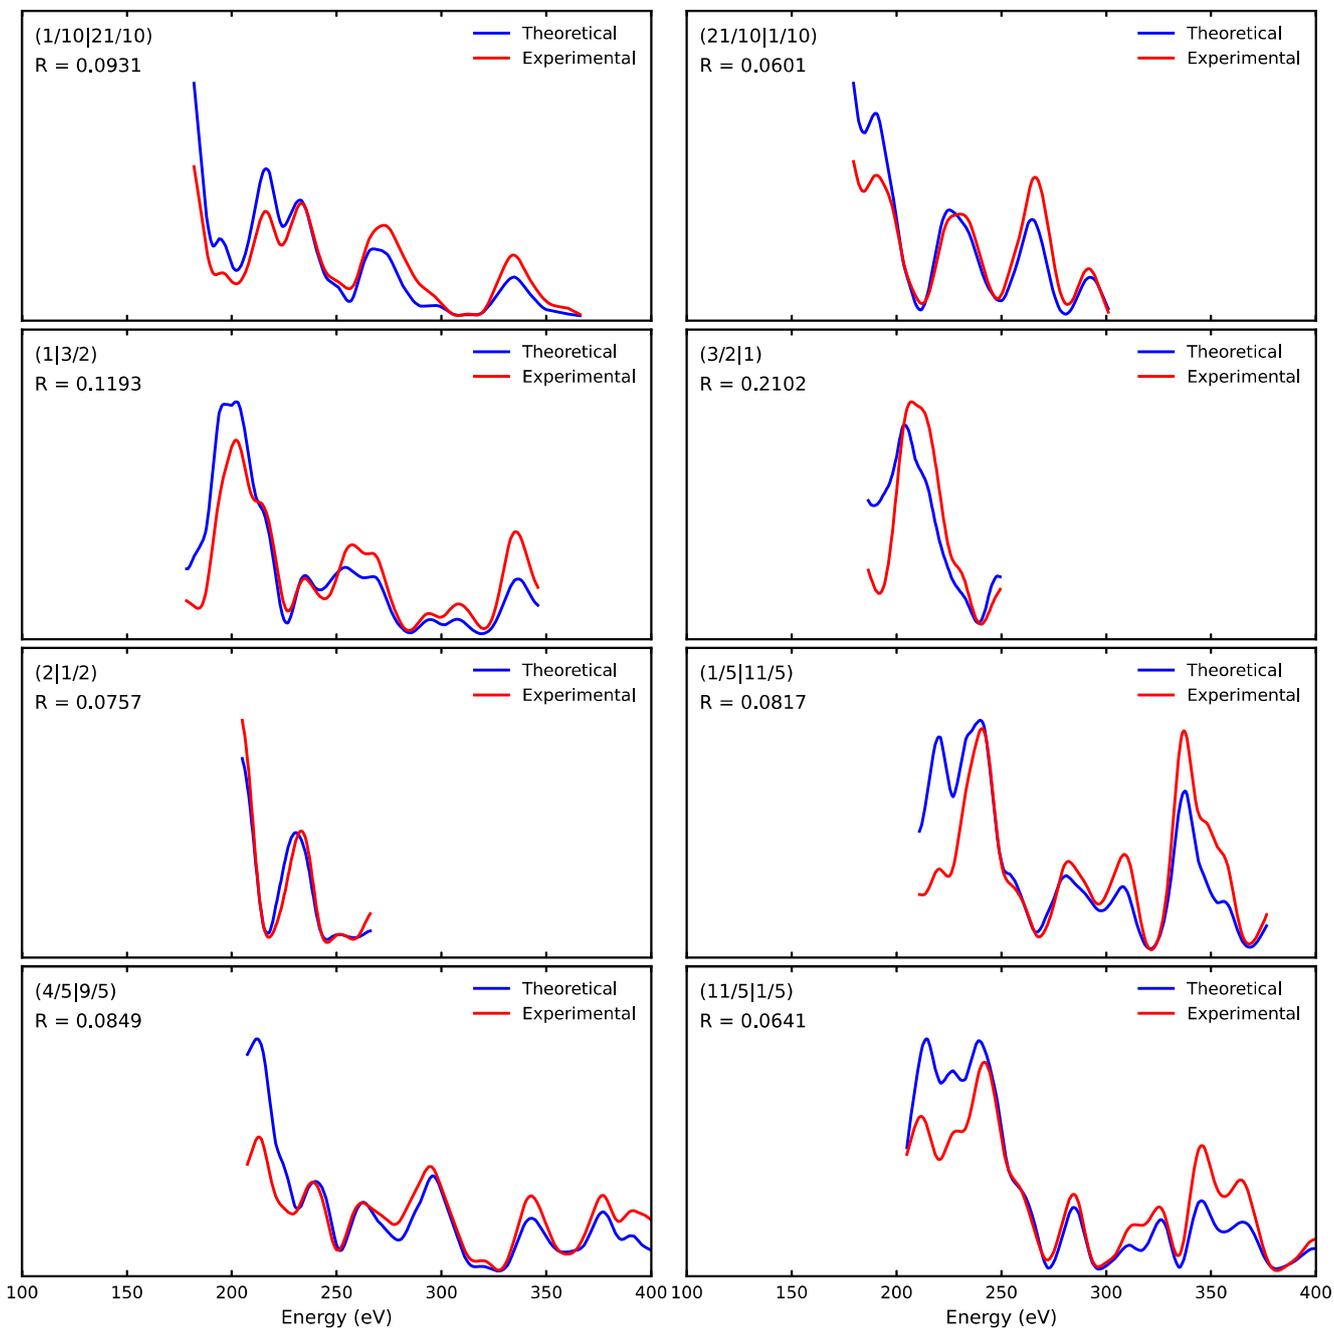

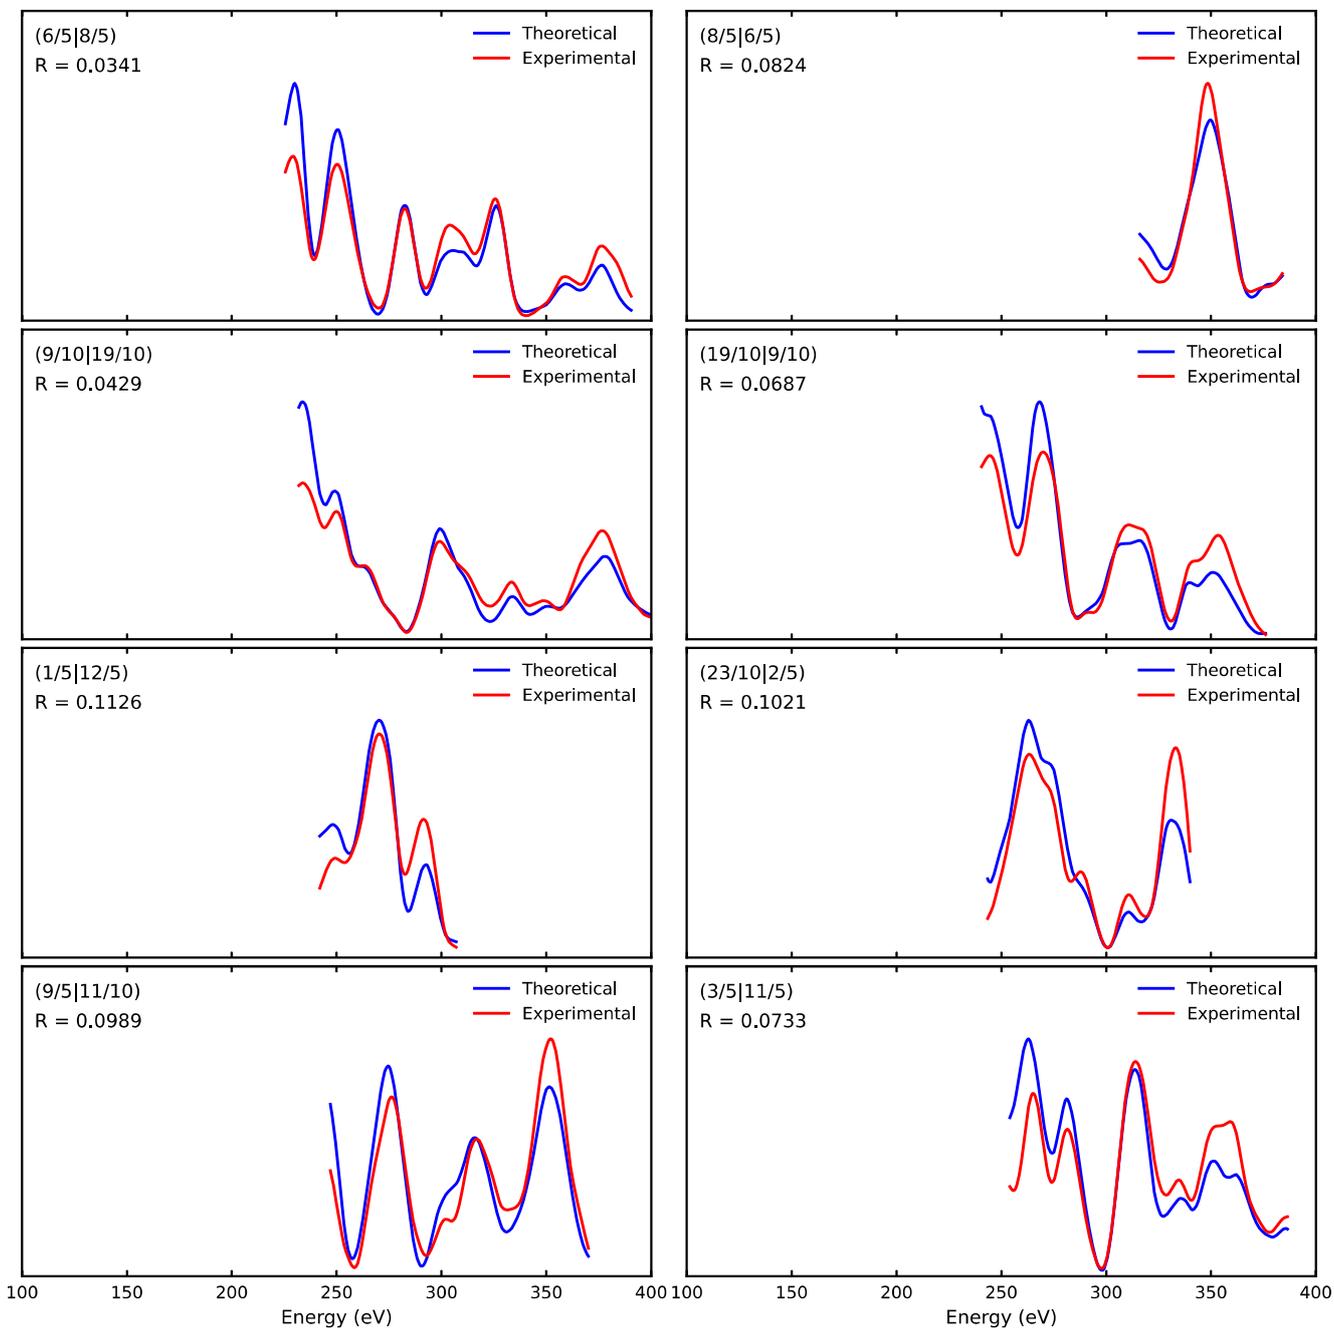

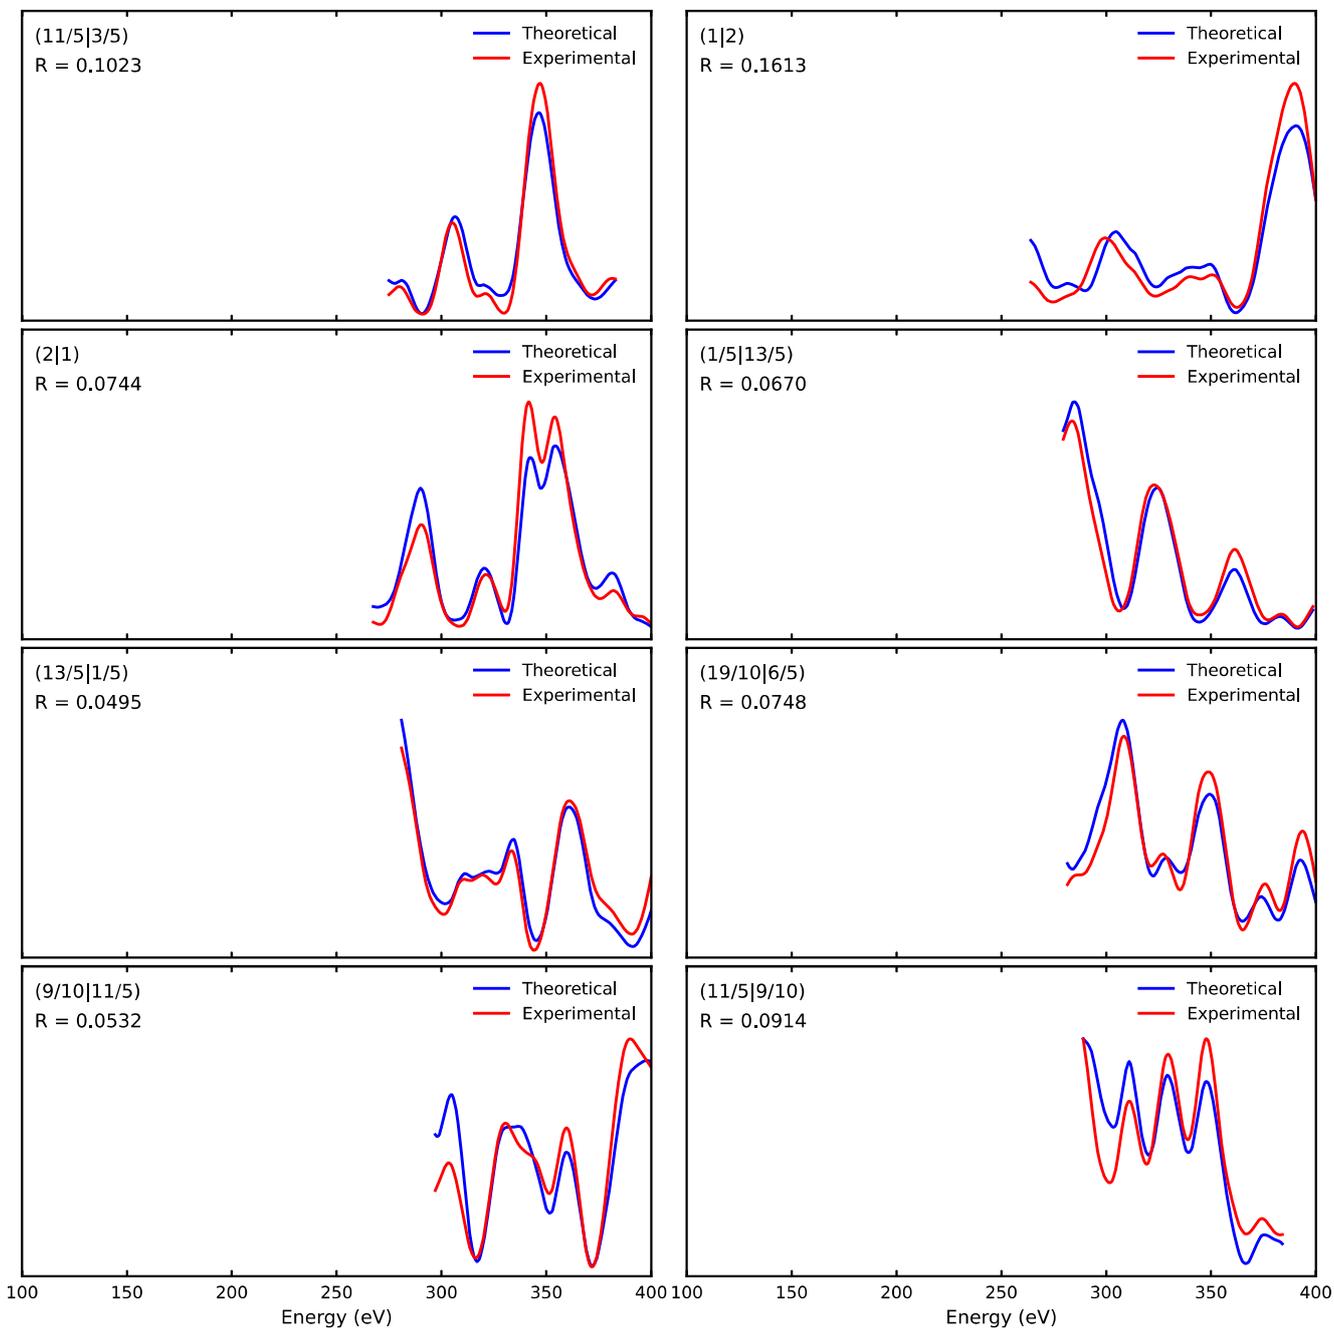

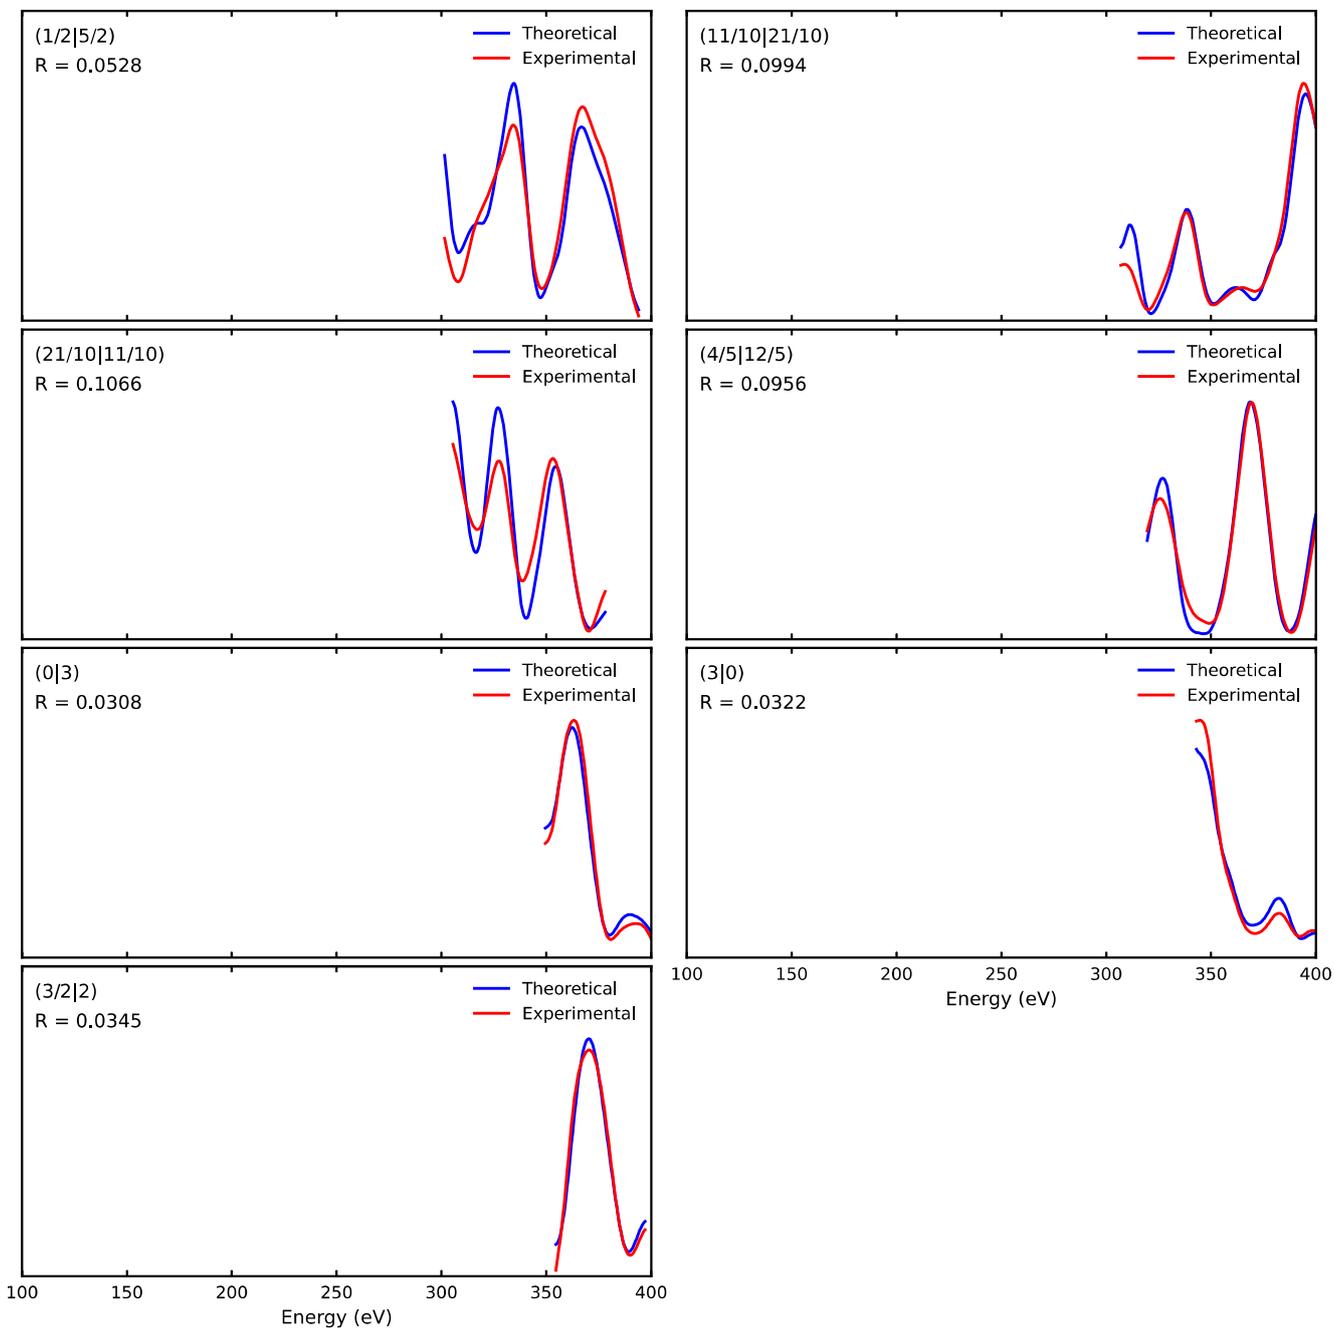

Supplement: Supplementary file 2 [file rfactor_plots_bestfit.pdf]
