# Supplementary material for: Growth and crystallographic structure of TiTe$_2$ on Au(111): From sub-monolayer structures to single- and multi-layer films
Source: arXiv:2602.16647 ancillary file (2026-02-18)

# Geometry

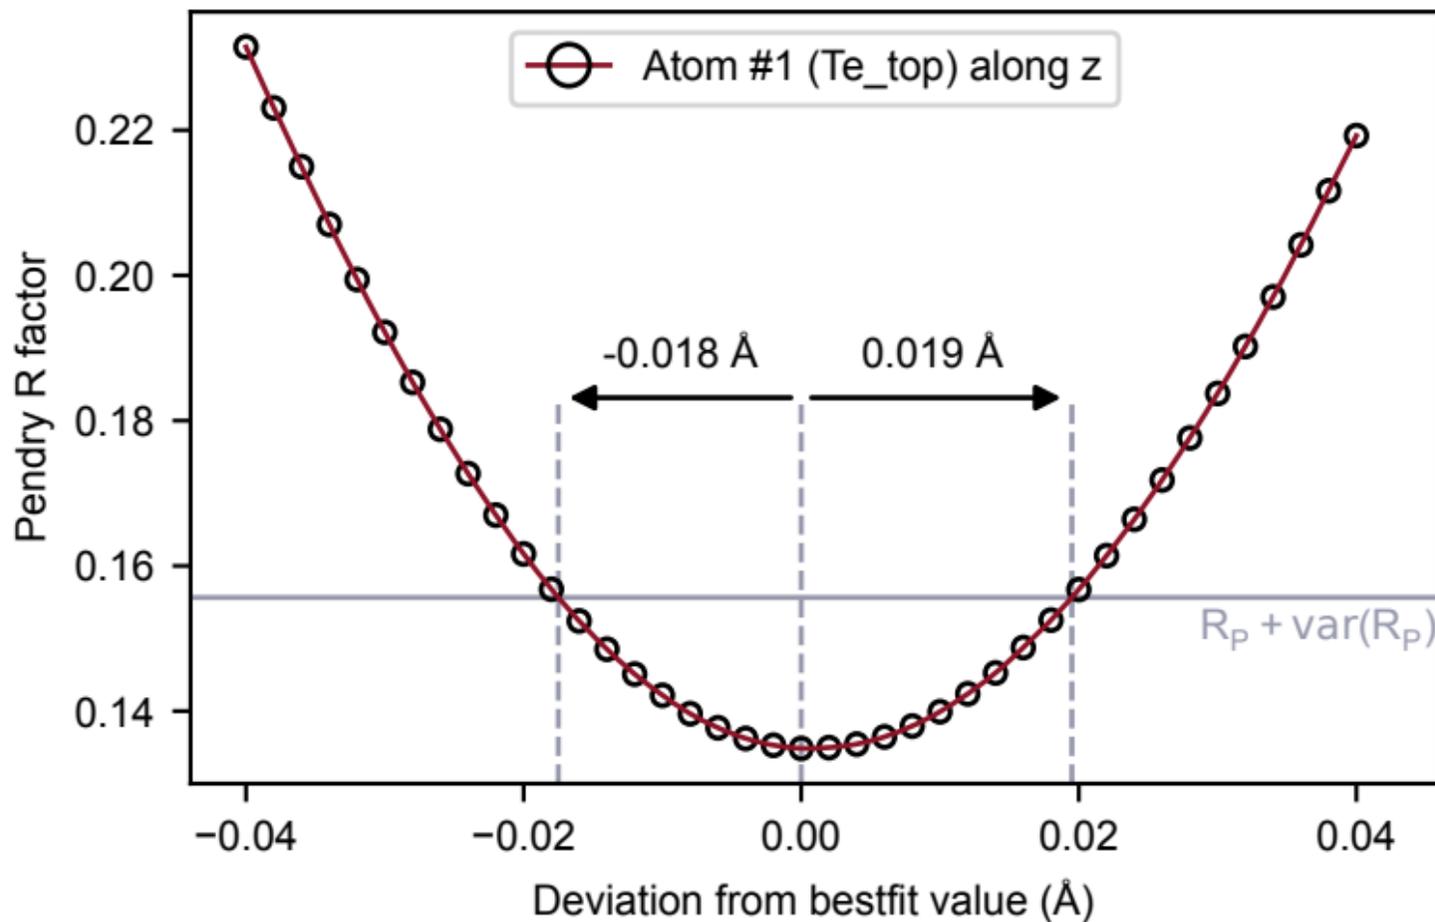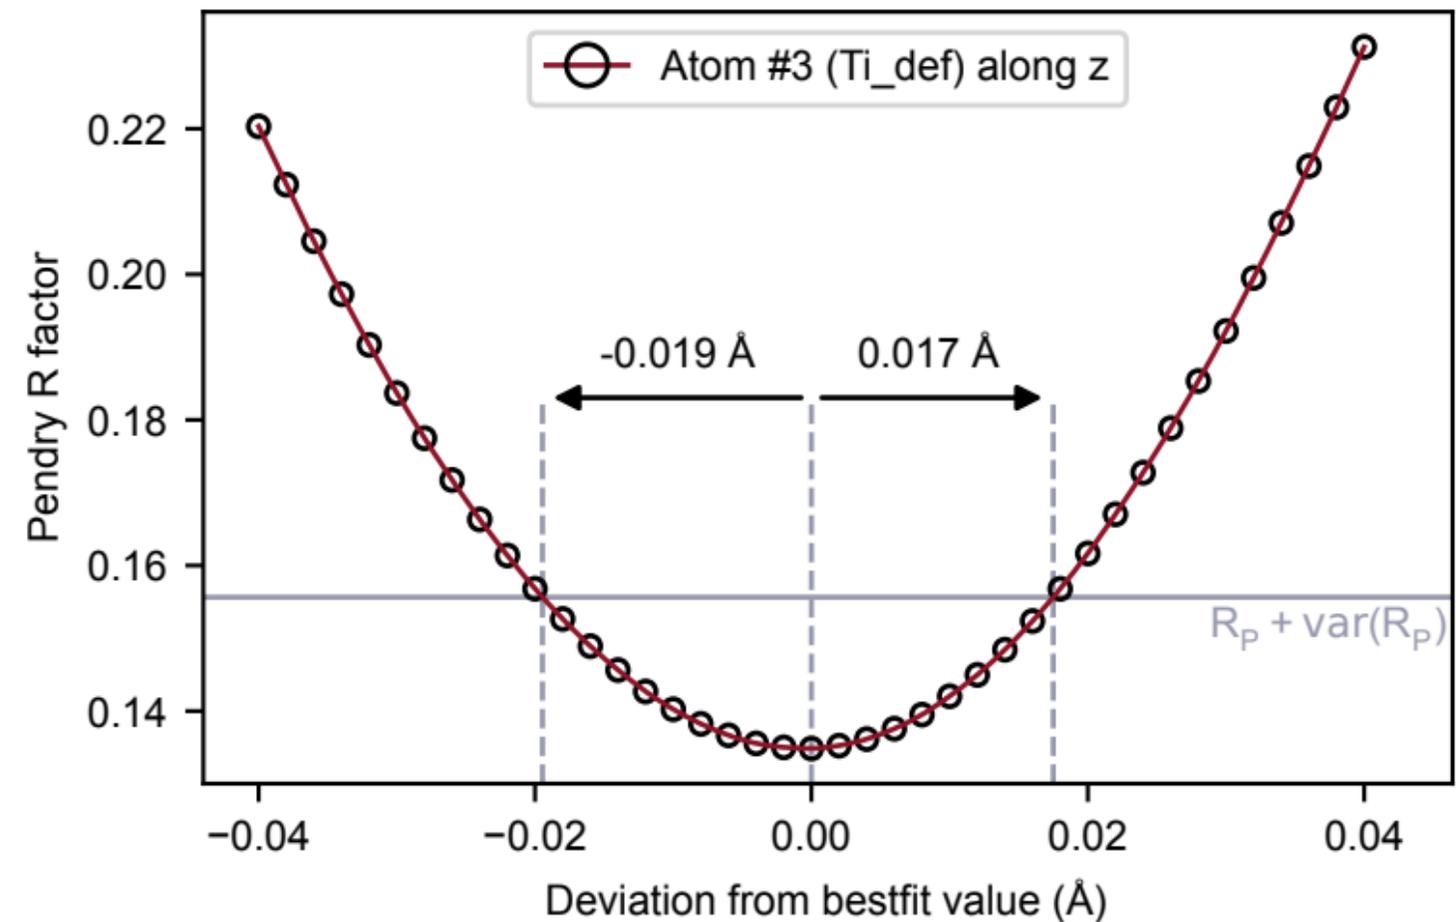

# Vibrational amplitudes

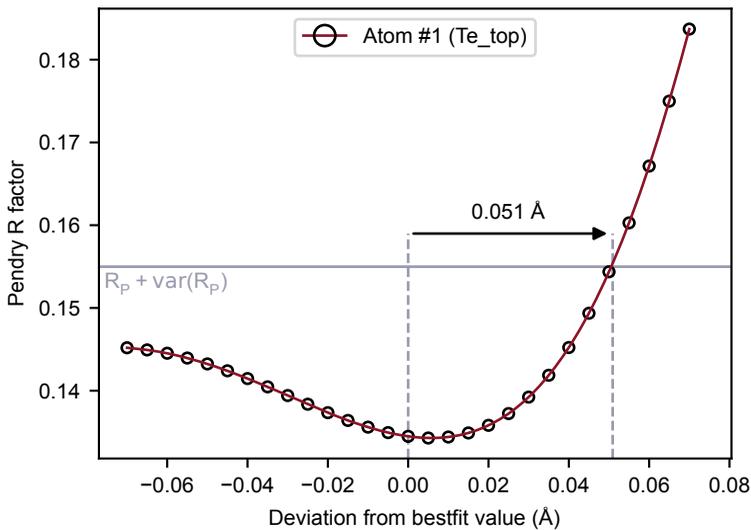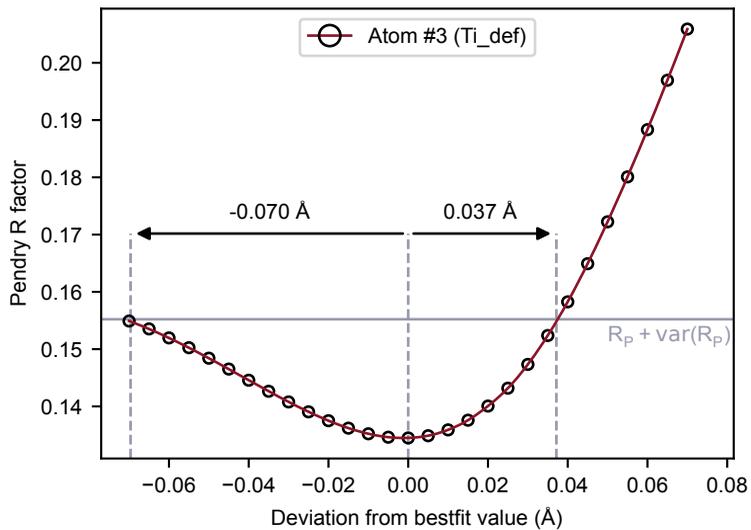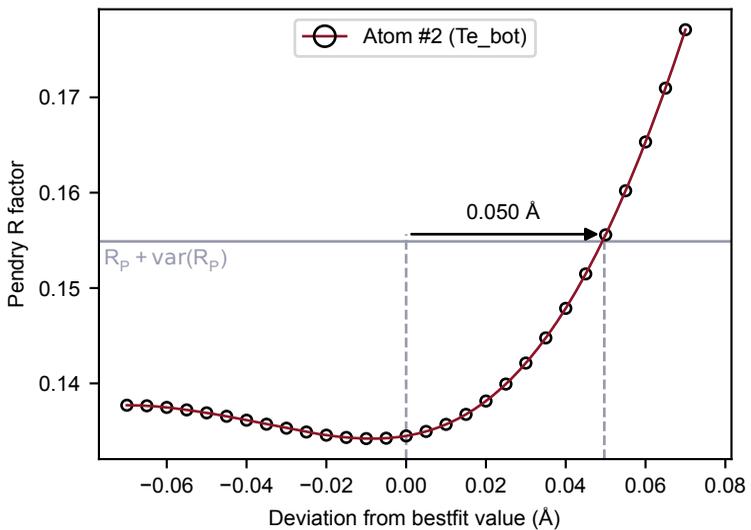

# Geometry

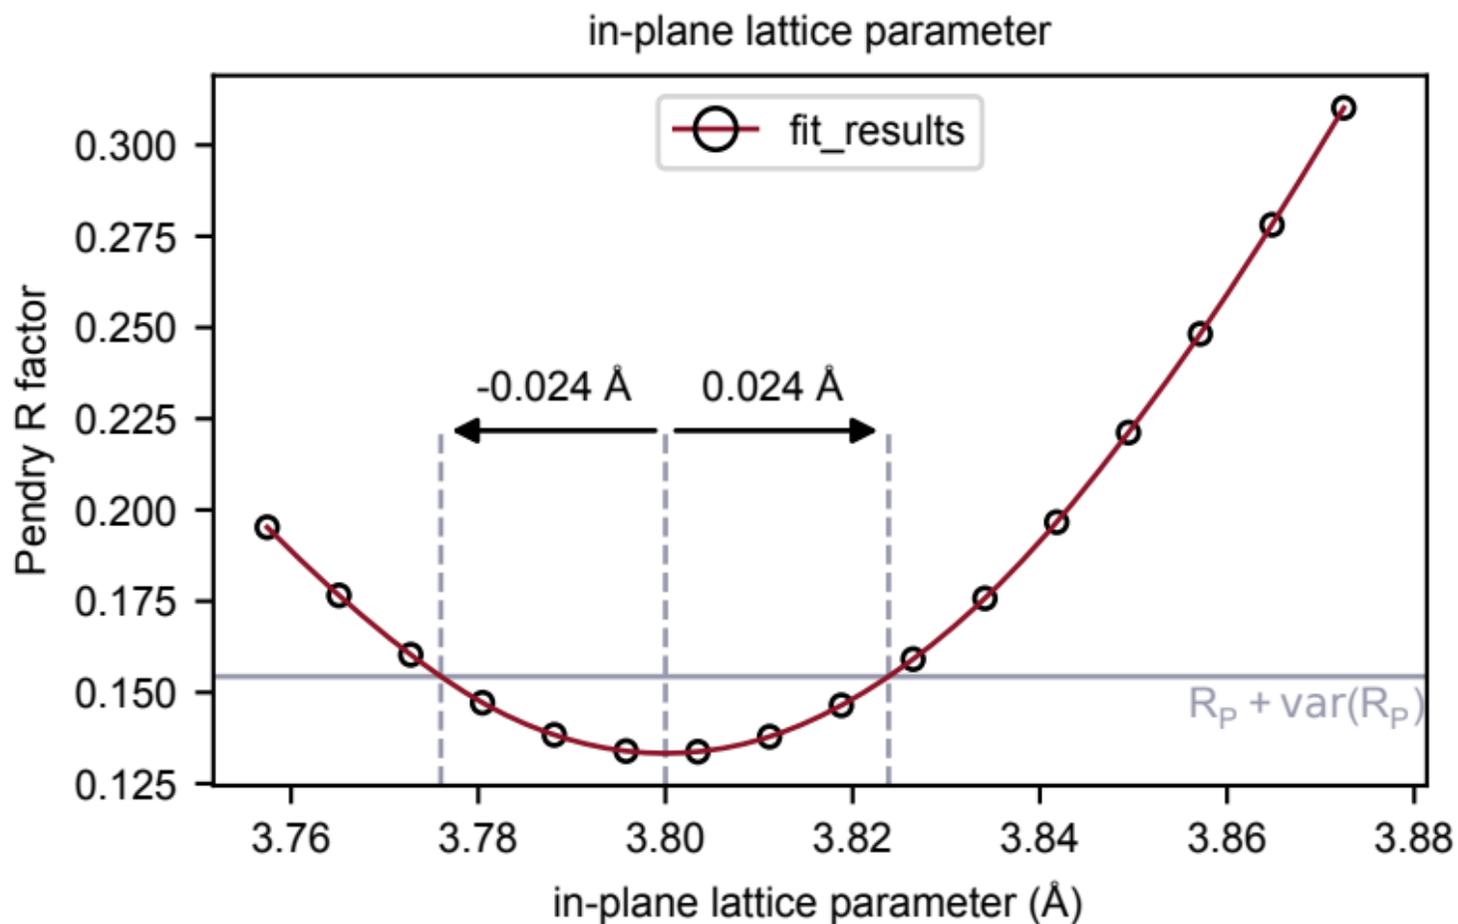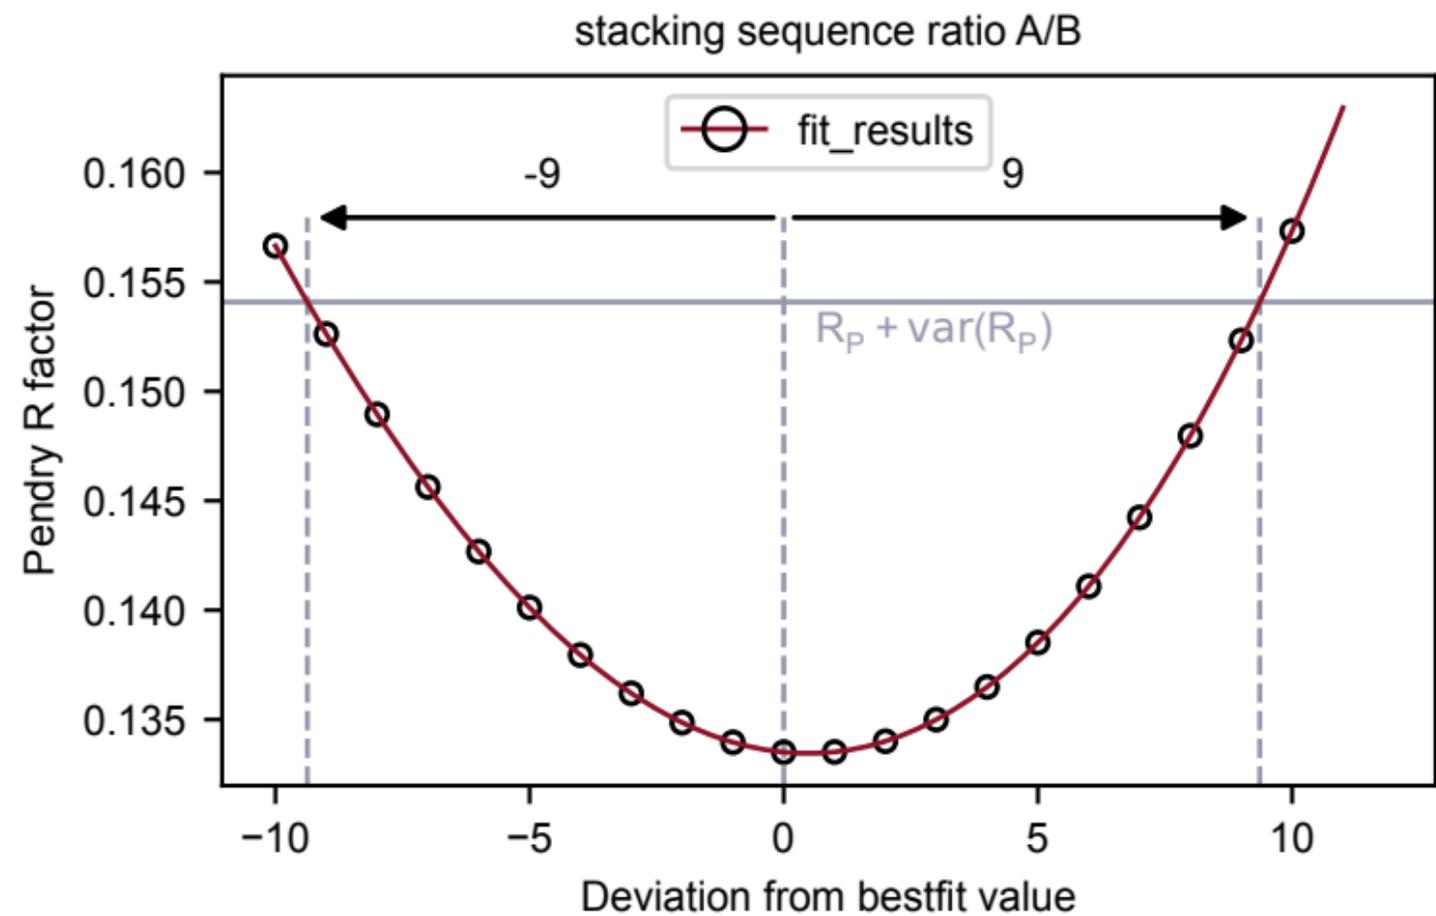

Supplement: Supplementary file 3 [file error_full-dynamic_singlelayer_tite2.pdf]
